# Supplementary material for: Extreme Sensitivity of Output Directionality to Boundary Perturbation in Wavelength-Scale Microcavities
Source: arXiv:1208.0792 source file (2012-08-03)
Supplement: Supplementary file 1 [file BDsensitivity_PartI_SI_July20.pdf]

# Supplemental material: Extreme sensitivity of output directionality to boundary perturbation in wavelength-scale microcavities

Li Ge,[1] Qinghai Song,[2] Brandon Redding,[3] and Hui Cao[3]

[1]*Department of Electrical Engineering, Princeton University, Princeton, NJ 08544, USA*
[2]*National Key Laboratory of Tunable Laser Technology, Institute of Opto-Electronics, Harbin Institute for Technology, Harbin, 150080, China*
[3]*Department of Applied Physics, Yale University, New Haven, CT 06520-8482, USA*

(Dated: August 3, 2012)

PACS numbers: 42.55.Sa,42.25.-p,05.45.Mt

## BIDIRECTIONAL EMISSION OF A QUADRUPLE CAVITY SLIGHTLY DEFORMED FROM A MICRODISK

In the main text we showed that the quasi-WG in a quadrupole cavity with $R = 1\,\mu$m and $\epsilon_2 = -0.01$ emits in the horizontal directions ($\theta = 0°$, $180°$). The output directionality can be understood intuitively: the curvature of the boundary is the highest at $\theta = 90°$, $270°$, so the direct tunneling of light undergoing total internal reflection at these places is also the strongest, giving rise to the bidirectional emission observed.

Besides this intuitive argument based on the boundary curvature, the bidirectional emission can also be understood as a wave interference effect using the perturbation theory. To the leading order, the quadruple deformation scatters light only into the $m \pm 2$ components because of the factor $F_{pm} = \epsilon_2/2\,\delta_{p,m\pm2}$ in $\alpha_p$ and $\mu_p$ (see Eqs. (2), (3) in the main text), where $m$ is the dominant angular momentum inside the cavity of the quasi-WG mode. Since the $m + 2$ component is tightly confined within the cavity, the farfield pattern is largely determined by the interference of the $m$ and $m - 2$ components. From Eqs. (2) and (3) in the main text we find that they are in-phase and their amplitudes are almost equal, thus the angular dependence of the farfield is roughly $\cos(m\theta) + \cos(m - 2)\theta$, which has an envelope proportional to $\cos\theta$ that suppresses the output in the vertical directions, leading to the bidirectional emission in the horizontal directions.

## LOW-Q MODES AT A SMALL $\epsilon_3$

In the main text we showed with the Husimi projection that Mode 1 is well above the triangular orbit in the SOS ("◁"), but it could couple to a low-$Q$ mode which is localized on the triangle orbit and have unidirectional emission [1]. However, it does not happen for Mode 1 as the nearest low-$Q$ mode (Mode 1′ in Fig. 4(a) of the main text) emits more or less symmetrically in the forward and backward directions, as shown in Fig. S2.

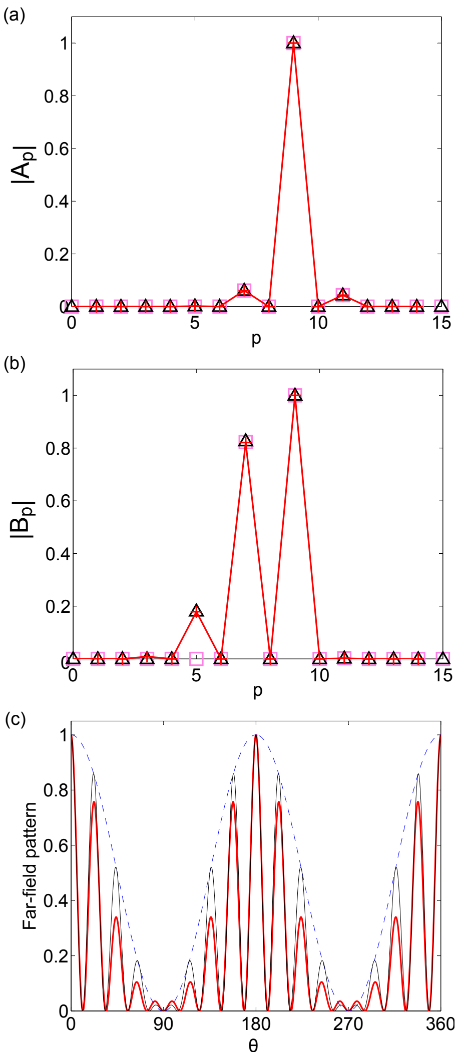


FIG. S1. Normalized Bessel (a) and Hankel (b) coefficients inside and outside the cavity (red crosses connected by solid line) of the resonance $kR = 4.387 - i1.809 \times 10^{-5}$ in a quadrupole cavity with $R = 1\,\mu$m, $\epsilon_2 = -0.01$, and $n = 3$. Squares and triangles show the results of the 1st and 2nd order perturbation theory, respectively. (c) Farfield intensity pattern of this mode (red solid line). 1st order perturbation result is given by the black solid line. 2nd order result overlaps with the numerical data. Blue dashed line shows the envelope function $(\cos\theta)^2$.

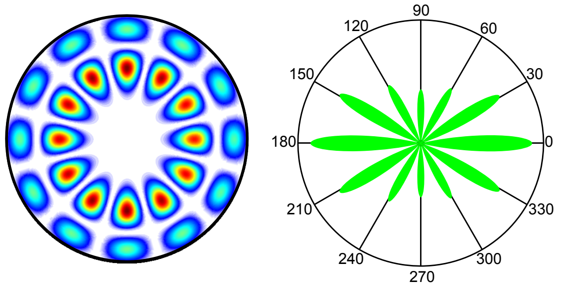


FIG. S2. Internal structure and farfield pattern of the low-Q resonance at $k'R = 4.391 - i2.019 \times 10^{-2}$ in a quadruple cavity with $R = 1\,\mu$m, $\epsilon_2 = -0.01$, $\epsilon_3 = 10^{-4}$, and $n = 3$.

## PERTURBATION THEORY FOR TE MODES

We adopt the perturbation theory for TM modes introduced in [2] to TE modes. The boundary conditions for TE modes

$$\psi_<(\rho,\theta) = \psi_>(\rho,\theta), \quad \frac{1}{n^2}\frac{\partial\psi_<}{\partial r} = \frac{\partial\psi_>}{\partial r}, \tag{1}$$

leads to a more complicated perturbation series and an additional first order correction. Here $\psi_{<(>)}(r,\theta)$ are the wave function inside (outside) the cavity. By expanding the above boundary conditions around $r = R$ and to the second order in $\epsilon$, we obtain

$$\psi_< - \psi_> = -\epsilon f(\theta)\left(\frac{\partial\psi_<}{\partial r} - \frac{\partial\psi_>}{\partial r}\right) - \frac{1}{2}\epsilon^2 f(\theta)^2\left(\frac{\partial^2\psi_<}{\partial r^2} - \frac{\partial^2\psi_>}{\partial r^2}\right), \tag{2}$$

$$\frac{1}{n^2}\frac{\partial\psi_<}{\partial r} - \frac{\partial\psi_>}{\partial r} = -\epsilon f(\theta)\left(\frac{1}{n^2}\frac{\partial^2\psi_<}{\partial r^2} - \frac{\partial^2\psi_>}{\partial r^2}\right) - \frac{1}{2}\epsilon^2 f(\theta)^2\left(\frac{1}{n^2}\frac{\partial^3\psi_<}{\partial r^3} - \frac{\partial^3\psi_>}{\partial r^3}\right). \tag{3}$$

All quantities here are evaluated at $r = R$. Using the ansatz

$$\begin{cases}\psi_<(r,\theta) = \sum_p a_p \frac{J_p(nkr)}{J_p(nkR)}\cos(p\theta), & r < \rho(\theta),\\ \psi_>(r,\theta) = \sum_p (a_p + b_p)\frac{H_p(kr)}{H_p(kR)}\cos(p\theta), & r > \rho(\theta),\end{cases} \tag{4}$$

we derive

$$\psi_< - \psi_> = -\sum_p b_p \cos(p\theta), \tag{5}$$

$$\frac{1}{n^2}\frac{\partial\psi_<}{\partial r} - \frac{\partial\psi_>}{\partial r} = k\sum_p\left[a_p T_p(kR) - b_p\frac{H_p'(kR)}{H_p(kR)}\right]\cos(p\theta). \tag{6}$$

By comparing the above expressions with the expansions (2) and (3), we see that all $a_{p\neq m}$ and $b_p$ are at least of order $\epsilon^1$, and we define $a_{p\neq m} \equiv \alpha_p\epsilon + \beta_p\epsilon^2 + O(\epsilon^3)$ and $b_p \equiv \mu_p\epsilon + \gamma_p\epsilon^2 + O(\epsilon^3)$. In the case of TM modes $\mu_p = 0$ as $\psi_< - \psi_>$ is at least of order $\epsilon^2$ [2] by substituting the corresponding equation of (3) into (2).

Using (4) we rewrite the differences on the right hand sides of Eqs. (5) and (6) as

$$\frac{\partial\psi_<}{\partial r} - \frac{\partial\psi_>}{\partial r} = k\sum_p\left[a_p S_p(kR) - b_p\frac{H_p'(kR)}{H_p(kR)}\right]\cos(p\theta), \tag{7}$$

$$\frac{\partial^2\psi_<}{\partial r^2} - \frac{\partial^2\psi_>}{\partial r^2} = -\frac{k}{R}\sum_p\left[S_p(kR) + kR(n^2-1)\right]a_p\cos(p\theta) + \frac{k}{R}\sum_p\left[\frac{H_p'(kR)}{H_p(kR)} - (\frac{p^2}{kR} - kR)\right]b_p\cos(p\theta), \tag{8}$$

$$\frac{1}{n^2}\frac{\partial^2\psi_<}{\partial r^2} - \frac{\partial^2\psi_>}{\partial r^2} = -\frac{k}{R}\sum_p\left[T_p(kR) + \frac{p^2}{n^2kR}(n^2-1)\right]a_p\cos(p\theta) + \frac{k}{R}\sum_p\left[\frac{H_p'(kR)}{H_p(kR)} - (\frac{p^2}{kR} - kR)\right]b_p\cos(p\theta), \tag{9}$$

$$\begin{aligned}\frac{1}{n^2}\frac{\partial^3\psi_<}{\partial r^3} - \frac{\partial^3\psi_>}{\partial r^3} = {}& \sum_p\left[kT_p(kR)(\frac{p^2+2}{R^2} - n^2k^2) - (n^2-1)k^3\frac{H_p'(kR)}{H_p(kR)} + \frac{3p^2}{n^2R^3}(n^2-1)\right]a_p\cos(p\theta)\\ &-\sum_p\left[k\frac{H_p'(kR)}{H_p(kR)}(\frac{p^2+2}{R^2} - k^2) - \frac{1}{R}(\frac{3p^2}{R^2} - k^2)\right]b_p\cos(p\theta).\end{aligned} \tag{10}$$

When deriving the last three expressions, we have used $J_p''(z) + \frac{1}{z}J_p'(z) + (1 - \frac{p^2}{z^2})J_p(z) = 0$ and its derivative, which give, for example,

$$\frac{J_p''(nkR)}{J_p(nkR)} = -\frac{1}{nkR}\frac{J_p'(nkR)}{J_p(nkR)} + (\frac{p^2}{n^2k^2R^2} - 1), \tag{11}$$

$$\frac{J_p'''(nkR)}{J_p(nkR)} = \frac{J_p'(nkR)}{J_p(nkR)}(\frac{p^2+2}{n^2k^2R^2} - 1) - \frac{1}{nkR}(\frac{3p^2}{n^2k^2R^2} - 1). \tag{12}$$

Next we expand the Bessel and Hankel functions around $k = k_0$. It is straightforward to see that the zeroth order term in (6) vanish, which is consistent with the right hand side of (3). In the discussion below we keep the terms in Eqs. (2) and (3) up to order $\epsilon^2$, and Eqs. (5-10) become

$$\psi_< - \psi_> = -\sum_p (\mu_p \epsilon + \gamma_p \epsilon^2)\cos(p\theta) + O(\epsilon^3), \tag{13}$$

$$\begin{aligned}\frac{1}{n^2}\frac{\partial \psi_<}{\partial r} - \frac{\partial \psi_>}{\partial r} &= \epsilon k_0 \left[ k_1 R T'_m(k_0R)\cos(m\theta) + \sum_{p\neq m} \alpha_p T_p(k_0R)\cos(p\theta) - \sum_p \mu_p \frac{H'_p(k_0R)}{H_p(k_0R)}\cos(p\theta)\right] \\ &+ \epsilon^2 [k_1^2 R T'_m(k_0R) + k_0 k_2 R T'_m(k_0R) + \frac{1}{2}k_0 k_1^2 R^2 T''_m(k_0R)]\cos(m\theta) \\ &- \epsilon^2 \sum_p \left[ k_1 \mu_p \frac{H'_p(k_0R)}{H_p(k_0R)} + k_0 \mu_p k_1 R \left[\frac{H'_p(z)}{H_p(z)}\right]'_{z=k_0R} + k_0 \frac{H'_p(k_0R)}{H_p(k_0R)}\gamma_p \right]\cos(p\theta), \\ &+ \epsilon^2 \sum_{p\neq m} \left[k_1 \alpha_p T_p(k_0R) + k_0 \alpha_p k_1 R T'_p(k_0R) + k_0 T_p(k_0R)\beta_p\right]\cos(p\theta) + O(\epsilon^3),\end{aligned} \tag{14}$$

$$\begin{aligned}\frac{\partial \psi_<}{\partial r} - \frac{\partial \psi_>}{\partial r} &= k_0 S_m(k_0R)\cos(m\theta) + \epsilon k_1 [S_m(k_0R) + k_0 R S'_m(k_0R)]\cos(m\theta) \\ &+ \epsilon k_0 \left[\sum_{p\neq m}\alpha_p S_p(k_0R) - \sum_p \mu_p \frac{H'_p(k_0R)}{H_p(k_0R)}\right]\cos(p\theta) + O(\epsilon^2),\end{aligned} \tag{15}$$

$$\frac{\partial^2 \psi_<}{\partial r^2} - \frac{\partial^2 \psi_>}{\partial r^2} = -\frac{k_0}{R}[S_m(k_0R) + k_0R(n^2-1)]\cos(m\theta) + O(\epsilon^1), \tag{16}$$

$$\begin{aligned}\frac{1}{n^2}\frac{\partial^2 \psi_<}{\partial r^2} - \frac{\partial^2 \psi_>}{\partial r^2} &= -(n^2-1)\frac{m^2}{n^2R^2}\cos(m\theta) - \epsilon k_0 k_1 T'_m(k_0R)\cos(m\theta) - \epsilon \sum_{p\neq m}\left[\frac{k_0}{R}T_p(k_0R) + \frac{p^2}{n^2R^2}(n^2-1)\right]\alpha_p \cos(p\theta) \\ &+ \epsilon \sum_p \left[\frac{k_0}{R}\frac{H'_p(k_0R)}{H_p(k_0R)} - (\frac{p^2}{R^2} - k_0^2)\right]\mu_p\cos(p\theta) + O(\epsilon^2),\end{aligned} \tag{17}$$

$$\frac{1}{n^2}\frac{\partial^3 \psi_<}{\partial r^3} - \frac{\partial^3 \psi_>}{\partial r^3} = (n^2-1)\left[\frac{3m^2}{n^2R^3} - k_0^3\frac{H'_m(k_0R)}{H_m(k_0R)}\right]\cos(m\theta) + O(\epsilon^1), \tag{18}$$

Henceforth we drop the arguments in the Bessel and Hankel functions and their derivatives. The first order terms of $\epsilon$ in (2) are then

$$-\sum_p \mu_p \epsilon \cos(p\theta) = -\epsilon f(\theta) k_0 S_m \cos(m\theta), \tag{19}$$

which gives the first order correction in $b_p$:

$$\mu_p = (k_0R) S_m F^{(1)}_{pm}, \tag{20}$$

where $F^{(\nu)}_{pm} = c_p \int_0^{2\pi} f^\nu(\theta)\cos(p\theta)\cos(m\theta)d\theta/(2\pi R^\nu)$ ($\nu = 1, 2$). We have dropped the superscript of $F^{(1)}_{pm}$ in the main text.

The first order terms of $\epsilon$ in (3) are

$$\begin{aligned}&\epsilon k_0 \left[T'_m k_1 R\cos(m\theta) + \sum_{p\neq m}\alpha_p T_p \cos(p\theta) - \sum_p \mu_p \frac{H'_p}{H_p}\cos(p\theta)\right] \\ &= \epsilon f(\theta)\frac{m^2}{n^2R^2}(n^2-1)\cos(m\theta),\end{aligned} \tag{21}$$

which give

$$k_1 R = \frac{1}{T'_m}\left[\frac{m^2}{n^2k_0R}(n^2-1) + k_0 R S_m \frac{H'_m}{H_m}\right]F^{(1)}_{mm}, \tag{22}$$

$$\alpha_{p\neq m} = \frac{1}{T_p}\left[\frac{m^2}{n^2k_0R}(n^2-1) + k_0 R S_m \frac{H'_p}{H_p}\right]F^{(1)}_{pm}. \tag{23}$$

Using $T_m = 0$, or $nH'_m/H_m = J'_m/J_m$, and the relation

$$T'_m = \left[\frac{J''_m}{J_m} - \left(\frac{J'_m}{J_m}\right)^2\right] - \left[\frac{H''_m}{H_m} - \left(\frac{H'_m}{H_m}\right)^2\right] \tag{24}$$

$$= -\frac{(n^2-1)m^2}{(nk_0R)^2} - \frac{H'_m}{H_m}S_m, \tag{25}$$

Eq. (22) is reduced to $k_1 = -k_0 F^{(1)}_{mm}$, which is the same as the 1st order correction of TM resonances [2].

The $\epsilon^2$ terms in (2) are

$$
\begin{aligned}
&-\sum_p \gamma_p \epsilon^2 \cos(p\theta)\\
&= -\epsilon f(\theta)\left[\epsilon\left(k_1 S_m + k_0 k_1 R S'_m - k_0\mu_m \frac{H'_m}{H_m}\right)\cos(m\theta)\right.\\
&\left. \quad +\epsilon k_0 \sum_{p\neq m}\left(\alpha_p S_p - \mu_p\frac{H'_p}{H_p}\right)\cos(p\theta)\right]\\
&\quad +\frac{k_0}{2R}\epsilon^2 f(\theta)^2\left[S_m + k_0R(n^2-1)\right]\cos(m\theta),
\end{aligned} \tag{26}
$$

from which the 2nd order correction in $b_p$ can be derived

$$
\begin{aligned}
\gamma_p &= \left(k_1 R S_m + k_0 k_1 R^2 S'_m - k_0 R\mu_m \frac{H'_m}{H_m}\right)F^{(1)}_{pm}\\
&\quad + k_0 R\sum_{q\neq m}\left(\alpha_q S_q - \mu_q \frac{H'_q}{H_q}\right)F^{(1)}_{pq}\\
&\quad - \frac{k_0 R}{2}\left[S_m + k_0R(n^2-1)\right]F^{(2)}_{pm}
\end{aligned} \tag{27}
$$

$$
\begin{aligned}
&= (n^2-1)(k_0R)^2\left[1 + n^2\left(\frac{H'_m}{H_m}\right)^2\right]F^{(1)}_{mm}F^{(1)}_{pm}\\
&\quad + (n^2-1)k_0R\sum_{q\neq m}\frac{1}{T_q}\left(S_q\frac{m^2}{n^2k_0R} + \frac{k_0R}{n}S_m\frac{J'_q}{J_q}\frac{H'_q}{H_q}\right)F^{(1)}_{qm}F^{(1)}_{pq}\\
&\quad - \frac{k_0R}{2}\left[S_m + k_0R(n^2-1)\right]F^{(2)}_{pm}.
\end{aligned} \tag{28}
$$

The $\epsilon^2$ terms in (3) are

$$
\begin{aligned}
&\epsilon^2[k_1^2 R T'_m + k_0 k_2 R T'_m + \frac{1}{2}k_0 k_1^2 R^2 T''_m]\cos(m\theta)\\
&+\epsilon^2\sum_{p\neq m,m'}\left[k_1\alpha_p T_p + k_0\alpha_p k_1 R T'_p + k_0 T_p\beta_p\right]\cos(p\theta)\\
&-\epsilon^2\sum_p\left[k_1\mu_p\frac{H'_p}{H_p} + k_0\mu_p k_1 R\left[\frac{H'_p}{H_p}\right]' + k_0\frac{H'_p}{H_p}\gamma_p\right]\cos(p\theta),\\
=&-\epsilon f(\theta)\frac{k_0}{R}[-(k_1R\epsilon)T'_m\cos(m\theta)\\
&-\sum_{p\neq m}(T_p + \frac{p^2}{n^2k_0R}(n^2-1))\alpha_p\epsilon\cos(p\theta)\\
&+\sum_p(\frac{H'_p}{H_p} - \frac{p^2}{k_0R} + k_0R)\mu_p\epsilon\cos(p\theta)]\\
&-\frac{1}{2}\epsilon^2 f(\theta)^2(n^2-1)\left[-k_0^3\frac{H'_m}{H_m} + \frac{3m^2}{n^2R^3}\right]\cos(m\theta),
\end{aligned} \tag{29}
$$

the left hand side of which can be simplified using Eq. (21). From the $mth$ harmonic on both sides we obtain the second order correction to the resonance

$$
\begin{aligned}
T'_m k_2 R &= -\frac{1}{2}(k_1R)^2 T''_m + \gamma_m\frac{H'_m}{H_m} + \mu_m k_1 R\left[\frac{H'_m}{H_m}\right]'\\
&\quad + \left[k_1 R T'_m - \frac{k_1}{k_0}\frac{m^2(n^2-1)}{n^2k_0R}\right]F^{(1)}_{mm}\\
&\quad + \sum_{p\neq m}(T_p + \frac{p^2}{n^2k_0R}(n^2-1))\alpha_p F^{(1)}_{mp}\\
&\quad - \sum_p(\frac{H'_p}{H_p} - \frac{p^2}{k_0R} + k_0R)\mu_p F^{(1)}_{mp}\\
&\quad + \frac{1}{2}(n^2-1)\left[(k_0R)^2\frac{H'_m}{H_m} - \frac{3m^2}{n^2k_0R}\right]F^{(2)}_{mm},
\end{aligned} \tag{30}
$$

and from the $pth$ harmonic on both sides we obtain the second order correction in $a_{p\neq m}$:

$$
\begin{aligned}
T_p\beta_p &= -\alpha_p k_1 R T'_p + \gamma_p\frac{H'_p}{H_p} + \mu_p k_1 R\left[\frac{H'_p}{H_p}\right]'\\
&\quad + \left[k_1 R T'_m - \frac{k_1}{k_0}\frac{m^2(n^2-1)}{n^2k_0R}\right]F^{(1)}_{pm}\\
&\quad + \sum_{q\neq m}(T_q + \frac{q^2}{n^2k_0R}(n^2-1))\alpha_q F^{(1)}_{pq}\\
&\quad - \sum_q(\frac{H'_q}{H_q} - \frac{q^2}{k_0R} + k_0R)\mu_q F^{(1)}_{pq}\\
&\quad + \frac{1}{2}(n^2-1)\left[(k_0R)^2\frac{H'_m}{H_m} - \frac{3m^2}{n^2k_0R}\right]F^{(2)}_{pm}.
\end{aligned} \tag{31}
$$

In the main text we have shown that the perturbation theory derived gives good agreement with numerical data, which are obtained from the scattering matrix approach. Here we give one simple example to check the validity of the derived perturbation corrections analytically: $f(\theta) = R$, i.e. a disk of radius $\rho = R(1+\epsilon)$, which leads to $F^{(1)}_{pm} = F^{(2)}_{pm} = \delta_{pm}$. The exact solution of the resonance $k$ can be easily obtained from scaling, i.e. $k = k_0R/(R+\epsilon R) \approx k_0(1-\epsilon+\epsilon^2) + O(\epsilon^3)$, which implies $k_1 = -k_0 = -k_0F^{(1)}_{mm}$, as given by Eq. (22), and $k_2 = k_0$. To confirm the later, we note that Eq. (30) takes the following form:

$$
\begin{aligned}
k_2 R T'_m &= -\frac{1}{2}(k_1R)^2 T''_m + k_1 R T'_m + \gamma_m\frac{H'_m}{H_m}\\
&\quad + \frac{1}{2}(n^2-1)\left[(k_0R)^2\frac{H'_m}{H_m} - \frac{3m^2}{n^2k_0R}\right] + \mu_m k_1 R\left[\frac{H'_p}{H_p}\right]\\
&\quad - \frac{k_1}{k_0}\frac{m^2(n^2-1)}{n^2k_0R} - (\frac{H'_m}{H_m} - \frac{m^2}{k_0R} + k_0R)\mu_m.
\end{aligned} \tag{32}
$$

Using

$$
T''_m = -\frac{T'_m}{k_0R} + \frac{2(n^2-1)m^2}{n^0(k_0R)^3} - 2\frac{H'_m}{H_m}S'_m, \tag{33}
$$

$$
\frac{H''_m(kR)}{H_m(kR)} = -\frac{1}{kR}\frac{H'_m(kR)}{H_m(kR)} + (\frac{m^2}{k^2R^2} - 1), \tag{34}
$$

the right hand side of Eq. (32) is reduced to $k_0RT'_m$, indicating that $k_2 = k_0$ as we have expected.

## EFFECT OF SURFACE ROUGHNESS

The boundary roughness can be treated as perturbation with a wide range of angular momenta, i.e. $\delta\rho(\theta) = R\sum_p \delta_p\cos(p\theta)$. For the large angular momentum ones, their perturbative contribution only occurs to Bessel and Hankel coefficients of large $p$ to the leading order. These components decay rapidly outside the cavity and have little effect on the farfield. The output pattern changes only with the small angular momentum terms in the boundary roughness. To investigate the effect of small $p$ components to a deterministic modification of the boundary, $\delta_p(p = 4, 5, \ldots, 8)$ with a random amplitude up to $10^{-3}$ are included when we vary $\epsilon_3$. We found that the output pattern is modified by the presence of these extra terms, but the sensitivity to $\epsilon_3$ survives. Fig. S3(a) shows one example of $\delta\rho(\theta)$, and from Fig. S3(b) we see that $U$ of

Mode 1 displays a similar sensitivity to $\epsilon_3$ as that without the surface roughness. In Fig. S3(c) we model the surface roughness in a different way. We include 30 Gaussian bumps and pits randomly distributed around the cavity, with a random amplitude up to 1nm and a full-width-at-half-maximum of 5°. Again the sensitivity of $U$ to $\epsilon_3$ can still be observed.

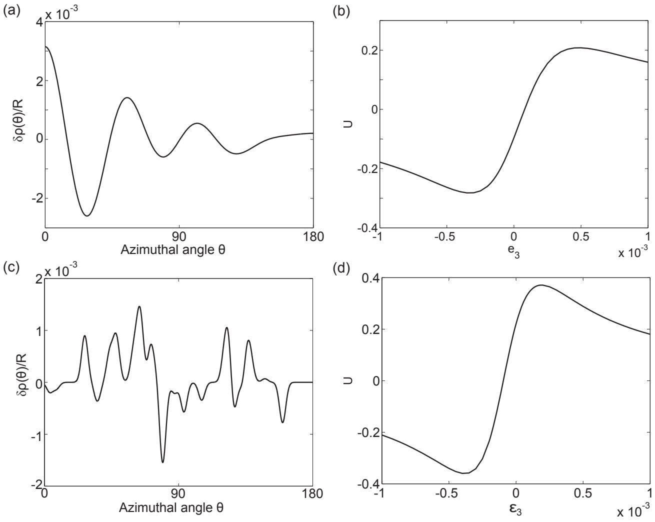


FIG. S3. (a) $\delta\rho(\theta)$ modeled as $R\sum_{p=4}^{8}\delta_p\cos(p\theta)$. In this example $\epsilon_4 = 0.4278\times10^{-3}$, $\epsilon_5 = 0.4814\times10^{-3}$, $\epsilon_6 = 0.8559\times10^{-3}$, $\epsilon_7 = 0.9886\times10^{-3}$, and $\epsilon_8 = 0.3936\times10^{-3}$. (b) $U$ of Mode 1 versus $\epsilon_3$ with the boundary roughness shown in (a). (c) $\delta\rho(\theta)$ modeled as random Gaussian bumps and pits. (d) $U$ of Mode 1 versus $\epsilon_3$ with the boundary roughness shown in (c). For simplicity we have assumed that $\delta\rho(\theta) = \delta\rho(-\theta)$ and only boundary roughness in $\theta \in [0, 180°]$ is shown in (a) and (c).

[1] Q. H. Song *et al.*, Phys. Rev. Lett. **105**, 103902 (2010).
[2] R. Dubertrand *et al.*, Phys. Rev. A **77**, 013804 (2008).
